# Supplementary material for: PointArena: Probing Multimodal Grounding Through Language-Guided Pointing
Source: arXiv:2505.09990 source file (2025-05-16)
Supplement: Supplementary file 1 [file 99-appendix.tex]

\appendix

\section{Appendix}
